# Supplementary material for: GRUtopia: Dream General Robots in a City at Scale
Source: arXiv:2407.10943 source file (2024-07-15)
Supplement: Supplementary file 1 [file APIs.tex]

\section{Learning-based Control APIs}

We conduct extensive evaluations of the locomotion controllers\footnote{The locomotion policies of quadruped robots and humanoid robots are trained using Isaac Gym. As the training procedures are related to other works currently under review, we will not expose the learning details here due to confidentiality policies. The implementations will be released in the future for the benefit of the community.} on both the Unitree H1 and Aliengo Z1 robots. These tests are carried out in two distinct environments: an open flat terrain and a cluttered, furniture-rich setting. In the locomotion controller tests, the robot is required to follow a collision-free trajectory. As shown in Tab.~\ref{tab:APIs}, the robot is tasked with adhering to predefined paths on flat terrain. Results indicate a perfect success rate and low following error in these controlled conditions. However, when transitioning to real-world applications, even with collision-free ground truth paths, there is a significant drop in performance. The manipulation tasks also revealed significant performance degradation when moving from controlled tests to more practical scenarios. This disparity underscores the challenges of transferring controlled environment successes to real-world scenarios.

Our findings indicate a crucial gap between the performance of current RL-trained locomotion controllers in controlled environments versus real-world scenarios. This gap is evident in both locomotion and manipulation tasks. Consequently, we advocate for a more integrated research approach, combining low-level control studies with high-level task execution in realistic settings.
