# Supplementary material for: GRUtopia: Dream General Robots in a City at Scale
Source: arXiv:2407.10943 source file (2024-07-15)
Supplement: Supplementary file 2 [file more_baselines.tex]

\begin{table}
\centering

\caption{\small
Experimental results of more baselines on Object Loco-Navigation and Social Loco-Navigation. (PL: Path Length, \textbf{SR}: Success Rate, SPL: Success rate weighted by normalized inverse Path Length, ECR: Excluded Candidate Rate, RT: Reset Times)
} % \caption
\vspace{1ex}
\resizebox{\linewidth}{!}{ %< auto-adjusts font size to fill line
\begin{tabular}{@{}|cc|cccc|cccc|ccccc|ccccc|@{}}
\hline
\multicolumn{2}{|c|}{\multirow{3}*{Method}} & \multicolumn{8}{c|}{Object Loco-Navigation} & \multicolumn{10}{c|}{Social Loco-Navigation}   \\
\cline{3-20}
~ & ~ & \multicolumn{4}{c|}{\texttt{validation}} & \multicolumn{4}{c|}{\texttt{test}} & \multicolumn{5}{c|}{\texttt{validation}} & \multicolumn{5}{c|}{\texttt{test}} \\
~ & ~ & PL & SR & SPL & RT & PL & SR & SPL & RT & PL & SR & SPL & ECR & RT & PL & SR & SPL & ECR & RT  \\
\hline

\multirow{2}*{\rotatebox{90}{VLM }} &\multicolumn{1}{|c|}{\multirow{2}*{InternVL-chat-1.5~\cite{chen2024far}}} & \multirow{2}*{12.77} & \multirow{2}*{8} & \multirow{2}*{5.45} & \multirow{2}*{0.67} & \multirow{2}*{10.85} & \multirow{2}*{5.5} & \multirow{2}*{3.88} & \multirow{2}*{0.23} & \multirow{2}*{15.19} & \multirow{2}*{0} &\multirow{2}*{ 0} & \multirow{2}*{0} & \multirow{2}*{6.67} & \multirow{2}*{16.80} & \multirow{2}*{0} & \multirow{2}*{0} & \multirow{2}*{0} & \multirow{2}*{6.35} \\
&\multicolumn{1}{|c|}{~}&&&&\multicolumn{1}{c|}{~}&&&&\multicolumn{1}{c|}{~}&&&&&\multicolumn{1}{c|}{~}&&&&&\multicolumn{1}{c|}{~}\\
\hline
\multirow{3}*{\rotatebox{90}{LLM }}&\multicolumn{1}{|c|}{Llama-3 8B~\cite{llama3}} & 25.97 & 10 & 7.21 & 0.84 & 23.32 & 15.5 & 10.96 & 0.57 & 20.77 & 5 & 3.49 & 17.69 & 1.54 & 21.42 & 11 & 6.26 & 7.21 & 1.89\\
~ &\multicolumn{1}{|c|}{InternLM-2-Chat~\cite{cai2024internlm2}} & 22.29 & 18 & 10.97 & 0.42 & 22.62 & 21.5 & 12.45 & 0.62 & 22.25 & 11 & 6.37 & 4.93 & 1.79 & 20.97 & 7.50 & 4.40 & 6.32 & 2.22\\
~ &\multicolumn{1}{|c|}{ChatGLM3~\cite{zeng2022glm}} & 22.75 & 22 & 12.97 & 0.60 & 23.78 & 22 & 11.68 & 0.74 & 21.13 & 8 & 4.61 & 7.1 & 2.06 & 20.36 & 11 & 6.97 & 0.13 & 2.25\\
\hline
\end{tabular}
} % \resizebox
\vspace{-3ex}
\label{tab:benchmark}
\end{table}
