# Supplementary material for: GRUtopia: Dream General Robots in a City at Scale
Source: arXiv:2407.10943 source file (2024-07-15)
Supplement: Supplementary file 3 [file scene_categories.tex]

\begin{longtable}{| m{4cm} | m{5cm} |}
\caption{Details of scene categories in GRScenes.}\label{tab:scene_categories} \\
\hline
\textbf{Main Category} & \textbf{Sub-category} \\ 
\hline
Office Space & Office \\
 & Lobby \\
 & Pantry \\
 & Reception Room \\
 & Lecture Hall \\
\hline
Dining Space & Private Room \\
 & Cafe \\
 & Cafeteria \\
 & Milk Tea Shop \\
 & Hot Pot Restaurant \\
 & Chinese Restaurant \\
 & Teahouse \\
 & Buffet Restaurant \\
 & Western Restaurant \\
 & Dessert Bakery \\
 & Open Kitchen \\
 & Back Kitchen \\
 & Barbecue Restaurant \\
 & Fast Food Restaurant \\
 & Noodle Shop \\
 & Tavern \\
\hline
Entertainment Space & E-sports Room \\
 & Bar \\
 & Chess Room \\
 & KTV \\
 & Beauty Salon \\
 & Billiard Room \\
 & Nail Salon \\
 & Children's Playground \\
 & Cinema \\
 & Foot Bath Shop \\
 & Hair Salon \\
 & Script Murder \\
 & Internet Cafe \\
\hline
Commercial Space & Clothing Store \\
 & Sales Office \\
 & Live Broadcast Room \\
 & Supermarket \\
 & Mall \\
 & Bookstore \\
 & Convenience Store \\
 & Jewelry Store \\
 & Tobacco and Alcohol Store \\
 & Flower Shop \\
 & Tea Shop \\
 & Outdoor Stall \\
 & Pet Shop \\
 & Glasses Shop \\
 & Fruit Shop \\
 & Vegetable Market \\
 & Snack Shop \\
 & Pharmacy \\
 & Market \\
 & Maternal and Infant Store \\
 & Wedding Photography \\
 & Digital Store \\
 & Toy and Gift Store \\
 & Furniture Store \\
 & Exhibition Hall \\
\hline
Public Space & Public Toilet \\
 & Library \\
 & Museum \\
 & Command Center \\
 & Dressing Room \\
 & Locker Room \\
 & Bank \\
 & Activity Room \\
 & Workshop \\
 & Service Center \\
 & Honor Room \\
 & Gas Station \\
 & Airport \\
 & Station \\
 & Indoor Parking Lot \\
 & Government Offices \\
 & Religious Culture \\
 & Hospital \\
\hline
Hotel Space & Hotel \\
 & Homestay \\
\hline
Educational Space & School \\
 & Kindergarten \\
 & Classroom \\
 & Laboratory \\
 & Reading Room \\
\hline
General Space & Staircase \\
 & Elevator \\
 & Lobby \\
 & Corridor \\
 & Rest Area \\
 & Dormitory \\
 & Party Building Room \\
 & Atrium \\
\hline
Sports Space & Gym \\
 & Swimming Pool \\
 & Stadium \\
 & Yoga Room \\
\hline

\end{longtable}
