# Supplementary material for: GRUtopia: Dream General Robots in a City at Scale
Source: arXiv:2407.10943 source file (2024-07-15)
Supplement: Supplementary file 4 [file clarifications.tex]

\section*{Clarifications}
We would like to clarify a few mistakes in the main paper. In Fig.~\red{3}, ``World Information Manager'' should be ``World Knowledge Manager'' as introduced in lines 154-164. The metrics ``EC'' and ``SC'' in Tab.~\red{2-4} should be ``ECR'' and ``SCR'' as defined in lines 252-257. We will update the numbers reported in Tab.~\red{2-4} accordingly in the revision.
