# Supplementary material for: GRUtopia: Dream General Robots in a City at Scale
Source: arXiv:2407.10943 source file (2024-07-15)
Supplement: Supplementary file 5 [file ablation_dialogue_round.tex]

\begin{wraptable}[10]{r}{7cm}
\centering

\vspace{-2.5ex}
\caption{\small
The impact of allowed dialogue rounds on agent performance.
} % \caption
\resizebox{\linewidth}{!}{ %< auto-adjusts font size to fill line
\begin{tabular}{@{}|c|ccccc|@{}}
\hline
\multicolumn{1}{|c|}{\multirow{2}*{Round}} & \multicolumn{5}{c|}{Social Loco-Navigation}  \\
\cline{2-6}
~ & PL & SR & SPL & EC & RT \\
\hline
0 & 16.26 & 14.00 & 8.64 & - & 2.48\\
1 & 17.50 & 24.00 & 11.71 & 0.7 & 2.80\\
2 & 17.85 & 14.00 & 8.75 & 0.3 & 3.04\\
3 & 18.61 & 18.00 & 11.06 & 0.26 & 2.60\\
4 & 17.51 & 14.00 & 9.52 & 6.67 & 2.38\\
\hline
\end{tabular}
} % \resizebox
\label{tab:dialogue}
\end{wraptable}
