# Supplementary material for: GRUtopia: Dream General Robots in a City at Scale
Source: arXiv:2407.10943 source file (2024-07-15)
Supplement: Supplementary file 6 [file ablation_oracle.tex]

\begin{table}
\centering

\caption{\small
Impact of oracle actions on agent's performance.
} % \caption
\vspace{0.5ex}
\resizebox{0.8\linewidth}{!}{ %< auto-adjusts font size to fill line
\begin{tabular}{@{}|c|c|cccc|ccccc|@{}}
\hline
\multirow{2}*{\#} & \multicolumn{1}{c|}{\multirow{2}*{Controller}} & \multicolumn{4}{c|}{Object Loco-Navigation} & \multicolumn{5}{c|}{Social Loco-Navigation}    \\
\cline{3-11}
~ & ~ & PL & SR & SPL & RT & PL & SR & SPL & ECR & RT \\
\hline
1 & RL-based & 23.82 & 8.00 & 4.26 & 0.89  \\
2 & Oracle &  \\
\hline
\end{tabular}
} % \resizebox
\vspace{-3ex}
\label{tab:oracle}
\end{table}
